# Supplementary material for: Linearly Convergent Frank-Wolfe with Backtracking Line-Search
Source: arXiv:1806.05123 source file (2022-09-08)
Supplement: Supplementary file 2 [file appendixB.tex]

\clearpage
